# Supplementary material for: Resonant light scattering by a slab of ultracold atoms
Source: arXiv:2409.04148 ancillary file (2024-09-06)
Supplement: Supplementary file 1 [file SM_ResonantLightScattering_v6_arxiv.pdf]

# Supplemental Material for: Resonant light scattering by a slab of ultracold atoms

R. Vatré, R. Lopes, J. Beugnon, and F. Gerbier
*Laboratoire Kastler Brossel, Collège de France,*
*ENS-Université PSL, Sorbonne Université, CNRS*
*11 place Marcelin Berthelot, 75005 Paris, France*
(Dated: September 6, 2024)

## I. EXPERIMENTAL DETAILS

### A. Preparation of a quasi-2D Bose gas

We prepare a quantum-degenerate 2D gas in a vertical optical lattice trap with a period of 4 µm. The trapping potential is approximately harmonic with trapping frequencies $(\omega_x, \omega_y, \omega_z) = 2\pi \times (26, 16, 1900)$ Hz. We transfer a 3D Bose-Einstein condensate of up to $4.5\times10^4$ $^{174}$Yb atoms into a single site of the lattice. The 2D dimensionless interaction parameter is $\widetilde{g} = \sqrt{8\pi}a_s/l_z \approx 0.075$, with the $s-$wave scattering length $a_s \approx 5$ nm and the vertical harmonic oscillator length $l_z = \sqrt{\hbar/(m\omega_z)} \simeq 0.17\,\mu$m. The calculated Thomas-Fermi chemical potential is $\mu_{\rm TF}/h \approx 1$ kHz$< \hbar\omega_z$, well in the 2D regime.

### B. Frequency scans

We use circularly-polarized light to drive the $\sigma^+$ Zeeman transition in an applied magnetic field varying from $B \simeq 40$ to $\simeq 200$ G. The atomic resonance frequency $\omega_0(B)$ for the $\sigma^+$ transition $J = 0, m_J = 0 \to J' = 1, m_{J'} = 1$ then varies linearly with $B$. For practical reasons, we perform frequency scans of the laser detuning $\widetilde{\delta} = 2(\omega_{\rm L} - \omega_0)/\Gamma_0$ by changing $B$, keeping the laser frequency fixed.

### C. Calibration of the atomic density

We use high-intensity absorption imaging [1, 2] to calibrate the atomic surface density $\rho_{\rm 2D}$. In high-intensity imaging, the probe transition is strongly saturated and multiple scattering is strongly suppressed, at the cost of a lower signal-to-noise ratio. For multi-level atoms, it is also necessary to use and calibrate a heuristic high intensity absorption cross-section accounting in an effective way for Raman scattering and optical pumping effects [1, 2]. These parasitic effects are absent for $^{174}$Yb atoms (or other atoms with a simple $J = 0 \leftrightarrow J = 1$ transition) where the absorption cross-section is known from first principles.

In practice, we use a probe intensity $I_{\rm L} \approx 28\, I_{\rm sat}$ and an imaging pulse time of $t_{\rm p} = 2$ µs. This procedure gives us a spatial map of the atomic density $\rho_{\rm 2D}(x, y)$ that we use to determine the average densities in each region of interest (ROI) for the light scattering measurements. ROIs are clustered around the cloud center. Regions of lower density near the cloud edge are typically not used because the spatial variations of the density cannot be neglected there. To extend the range of our measurements towards low densities, we reduce the atom number (thus the peak atomic density) in a controlled way by applying a pulse of resonant light to the 3D BEC before loading it into the final 2D trap.

We fit the surface densities $\rho_{\rm 2D}(x, y)$ using the known equation of state of a 2D Bose gas [3]. This fit allows us to assign a chemical potential and a temperature to each cloud. We typically obtain temperatures in the range $40 - 70$ nK, well below the 2D degeneracy temperature $T_{\rm 2D} \approx 170$ nK [4]. For such low temperatures, we expect that quantum statistical effects, as studied in [5] and recently measured in [6] for a 3D gas near the transition temperature, are negligible.

### D. Atomic motion

We consider first the momentum distribution of the initial state. An atom in the ground state of the vertical trap has a typical velocity $v_z = \hbar/ml_z$, which gives a Doppler shift of the probe transition $\Delta\omega_0 = \hbar k_0/ml_z \sim 10^{-3}\Gamma$. Transverse motion leads to even smaller Doppler shifts, and we therefore ignore the impact of the initial momentum distribution on the optical response.

The probe beam modifies the momentum distribution through radiation pressure and momentum diffusion. These two effects impose upper limits to the pulse duration. In a classical picture, the atoms acquire an average velocity $v_z \simeq F_{\rm rad}t_{\rm p}/m$ in the vertical direction due to the radiation pressure force $F_{\rm rad} \simeq \Gamma\hbar k_{\rm L}s/2$, with $s = I_{\rm L}/I_{\rm sat}$ the saturation parameter. Requiring that the associated Doppler shift $k_{\rm L}v_z$ remains much smaller than $\Gamma$, we arrive at the condition

$$t_{\rm p} \ll \frac{2m}{s\hbar k_{\rm L}^2} \approx 24\,\mu{\rm s}. \quad (1)$$

We verify this condition experimentally by choosing $t_{\rm p} = 5$ µs. We also check that momentum diffusion has a negligible effect on the imaging resolution. Momentum diffusion in the transverse plane leads to a momentum broadening $\Delta p_\perp \approx \hbar k_{\rm L}\sqrt{\frac{\Gamma t_{\rm p} s}{6}}$. We estimate the transverse spatial diffusion by the displacement $d_\perp \approx t_{\rm p}\Delta p_\perp/m \approx 0.1$ µm. Since $d_\perp$ is smaller than the effective size $\approx 0.5$ µm of one pixel of the camera in the object plane, transverse diffusion caused by the probe beam is negligible.

## II. IMAGE ANALYSIS

We give here the details of the analysis of images as in Fig. 1b in the main text. The optical intensity at a point $\boldsymbol{r}$ can be written

$$I(\boldsymbol{r}) = \left|t(\boldsymbol{r})\boldsymbol{E}_1(\boldsymbol{r}) + \boldsymbol{E}_2(\boldsymbol{r})\right|^2 = (\eta T(\boldsymbol{r}) + 1) I_{\mathrm{L}}(\boldsymbol{r}) \left\{1 + \frac{2\sqrt{\eta T(\boldsymbol{r})}}{\eta T(\boldsymbol{r}) + 1}\left|\boldsymbol{\epsilon}_2^* \cdot \boldsymbol{\epsilon}_1\right| \cos\left[qx + \Phi(\boldsymbol{r}) + \Delta\phi(\boldsymbol{r})\right]\right\}. \quad (2)$$

Here $t(\boldsymbol{r}) = \sqrt{T(\boldsymbol{r})}\mathrm{e}^{\mathrm{i}\Delta\phi(\boldsymbol{r})}$ is the complex transmission of the atomic medium, $\boldsymbol{E}_{1/2}$ (respectively, $\boldsymbol{\epsilon}_{1/2}$) denote the electric fields (resp., polarization vectors) of the probe or reference wave, and $I_{\mathrm{L}} = |\boldsymbol{E}_2|^2$ is the intensity profile of the reference wave. The intensity imbalance $\eta = |\boldsymbol{E_1}|^2/|\boldsymbol{E_2}|^2 \approx 0.95$ and the relative phase $\Phi(\boldsymbol{r})$ are introduced by the propagation through the optical system, independently of the presence or absence of atoms.

For each image, we define several rectangular regions of interest (ROI) of size $\approx 4.6 \times 2.3\,\mu\mathrm{m}^2$ in the plane of the atoms centered around fixed positions $\boldsymbol{r}_\alpha$. The size of the ROIs is chosen large enough to average out photon shot noise, and small enough that the density can be considered uniform to better than 10 % across each ROI. Using the calibration procedure described in Section I C, we assign a particular 2D density $\rho_\alpha \equiv \rho_{\mathrm{2D}}(\boldsymbol{r}_\alpha)$ to each ROI $\alpha$. Integrating over the $y$-direction, we obtain fringe profiles $S_\alpha(x)$ as shown in Fig. 1(c) in the main text.

For each region $\alpha$, we fit the fringe profiles $S_\alpha(x)$ with the function

$$S_\alpha(x) = A_\alpha\left[1 + \gamma_\alpha \cos(qx + \phi_\alpha)\right]. \quad (3)$$

The mean optical intensity $A_\alpha$, the fringe contrast $\gamma_\alpha \in [0,1]$ and the local phase $\phi_\alpha$ are related to the parameters above through

$$A_\alpha = (1 + \eta T_\alpha) I_{\mathrm{L}}(\boldsymbol{r}_\alpha), \quad (4)$$

$$\gamma_\alpha = \frac{2\sqrt{\eta T_\alpha}}{1 + \eta T_\alpha}\left|\boldsymbol{\epsilon}_2^* \cdot \boldsymbol{\epsilon}_1\right|, \quad (5)$$

$$\phi_\alpha = \zeta(\boldsymbol{r}_\alpha) + \Delta\phi_\alpha. \quad (6)$$

We also define for each image a larger $46 \times 4.6\,\mu\mathrm{m}^2$ reference region centered around $\boldsymbol{r}_0$. As for the ROIs, the integrated fringe profile $S_{\mathrm{ref}}(x)$ is analyzed by fitting with the function

$$S_{\mathrm{ref}}(x) = A_{\mathrm{ref}}\left[1 + \gamma_{\mathrm{ref}} \cos(qx + \phi_{\mathrm{ref}})\right], \quad (7)$$

with

$$A_{\mathrm{ref}} = (1 + \eta) I_{\mathrm{L}}(\boldsymbol{r}_0), \quad (8)$$

$$\gamma_{\mathrm{ref}} = \frac{2\sqrt{\eta}}{1 + \eta}\left|\boldsymbol{\epsilon}_2^* \cdot \boldsymbol{\epsilon}_1\right|, \quad (9)$$

$$\phi_{\mathrm{ref}} = \zeta(\boldsymbol{r}_0). \quad (10)$$

In general, $\zeta(\boldsymbol{r}_0) \neq \zeta(\boldsymbol{r}_\alpha)$ and $I_{\mathrm{L}}(\boldsymbol{r}_0) \neq I_{\mathrm{L}}(\boldsymbol{r}_\alpha)$. To correct for these spatial inhomogeneities of the probe, we also record a second "background" image in the same conditions as the main one but without atoms in order to perform flat-field corrections. We indicate the quantities extracted from the background image with a prime subscript in the following. This additional background image would not be necessary if the probe intensity were spatially uniform and constant in time. In practice, neither is true. However, intensity variations between the main and background image are essentially due to power fluctuations of the probe laser which give a global multiplicative change of the entire profile. In that case, the ratio $A_\alpha/A_{\mathrm{ref}} = I_{\mathrm{L}}(\boldsymbol{r}_\alpha)/I_{\mathrm{L}}(\boldsymbol{r}_0)$ for the main image and $A'_\alpha/A'_{\mathrm{ref}} = I'_{\mathrm{L}}(\boldsymbol{r}_\alpha)/I'_{\mathrm{L}}(\boldsymbol{r}_0)$ for the background image are equal.

### 1. *Phase shift $\Delta\phi_\alpha$*

We extract straighforwardly the phase shift due to the atomic sample using

$$\Delta\phi_\alpha = \xi_\alpha - \xi_{\mathrm{ref}} - (\xi'_\alpha - \xi'_{\mathrm{ref}}). \quad (11)$$

### 2. *Intensity transmission $T_\alpha$*

The contrast $\gamma_\alpha$ and the mean intensity $A_\alpha$ provide two independent ways of inferring the intensity transmission coefficient $T_\alpha$ of ROI $\alpha$. The extraction methods are a bit more involved than for the phase shift, and we consider them in details.

*a. From the fringe contrast $\gamma$:* From Eqs. (5,9), we find the ratio

$$c = \frac{\gamma_\alpha}{\gamma_{\mathrm{ref}}} = \frac{(1+\eta)\sqrt{T_\alpha}}{1 + \eta T_\alpha}. \quad (12)$$

Solving for $T_\alpha$, we obtain

$$T_\alpha^{(\gamma)} = \eta\, h\left(\frac{2c\sqrt{\eta}}{1+\eta}\right) \quad (13)$$

with $h(x) = \left(1 - \sqrt{1 - x^2}\right)^2/x^2$. Note that the function $h$ becomes very steep when its argument is close to 1.

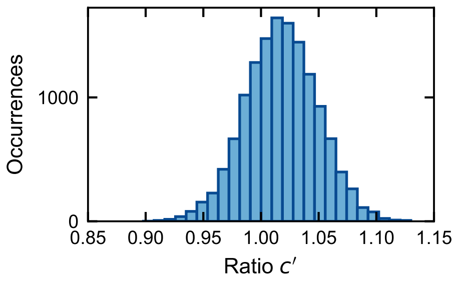


FIG. S1. Histogram of the measured values of $c' = \frac{\gamma'_\alpha}{\gamma'_{\rm ref}}$, the ratio of the fringe contrast in the ROI and in the reference regions, for *background images without atoms.* The histogram is peaked around one with a width of a few percents compatible with imaging noise (see Table I and Section V B). The observation that $c' \approx 1$ indicates that the assumptions behind our model to perform flat field correction are valid at the level of a few percents.

As a result, the present method is easily contaminated by experimental noise when the intensity transmission is close to 1 (*i.e.* for optically dilute sample).

Eq. (13) relies on assumptions about the spatial variations and temporal reproducibility of the probe intensity profile. As a check of these assumptions, we note that Eq. (13) applied to background images with $T_\alpha = 1$ leads to a contrast ratio $c' = 1$. We plot an histogram of the observed values of $c'$ in Fig. S1. We find that this ratio is indeed close to one, with fluctuations that are indicative of the level of imaging noise (see Section V B below) and of the relative error induced by this noise of the atomic quantities $T, \Delta\phi$.

*b. From the total intensity A:* For the main image containing the atoms, the ratio between the mean intensities in ROI $\alpha$ and in the reference region is

$$\frac{A_\alpha}{A_{\rm ref}} = \frac{T_\alpha + \eta}{1+\eta}\frac{I_1(\boldsymbol{r}_\alpha)}{I_1(\boldsymbol{r}_0)}. \tag{14}$$

For the background image, we have $A'_{\rm ref} = (1+\eta)I'_{\rm L}(\boldsymbol{r}_0)$, $A'_\alpha = (1+\eta)I'_{\rm L}(\boldsymbol{r}_\alpha)$ and $A'_\alpha/A'_{\rm ref} = I'_{\rm L}(\boldsymbol{r}_\alpha)/I'_{\rm L}(\boldsymbol{r}_0) = I_{\rm L}(\boldsymbol{r}_\alpha)/I_{\rm L}(\boldsymbol{r}_0)$ according to the discussion above. As a result, the transmission can be inferred by evaluating

$$T_\alpha^{(A)} = (1+\eta)\frac{A_\alpha A'_{\rm ref}}{A_{\rm ref}A'_\alpha} - \eta. \tag{15}$$

### A. Fits to the transmission and phase shift lines

To quantify a potential lineshift or line broadening, we fit the transmissions $T_\alpha^{(\gamma/A)}$ to Lorentzian functions

$$T_{\rm fit}(\widetilde{\delta}) = \frac{T_{\rm min}}{1 + \frac{(\widetilde{\delta}-\widetilde{\delta}_0)^2}{\zeta^2}}, \tag{16}$$

and the phase shifts $\Delta\phi_\alpha$ to dispersive functions

$$\Delta\phi_{\rm fit}(\widetilde{\delta}) = -\frac{\mathcal{A}_\phi}{2} \times \frac{\frac{\widetilde{\delta}-\widetilde{\delta}_0}{\zeta}}{1 + \frac{(\widetilde{\delta}-\widetilde{\delta}_0)^2}{\zeta^2}}, \tag{17}$$

with $\widetilde{\delta}_0$ describing a line shift and $\zeta$ a line broadening (both quantities are expressed in units of $\Gamma_0/2$). Fig. S2 shows the fitted $\widetilde{\delta}_0$ and $\zeta$ versus the surface density $\widetilde{\rho}_{\rm 2D}$. We observe the absence of line broadening and of a significant line shift. We believe the apparent line shift in the transmission data $T^{(\gamma)}$ is an artifact of the experimental analysis where small systematic errors are enhanced by the steepness of the $h$ function.

## III. COUPLED DIPOLE MODEL

### A. Foldy-Lax equations

We consider an ensemble of $N$ atoms coupled to the quantized electromagnetic (e-m) field. Each atom has a $J=0$ ground state $|g\rangle$ and a $J=1$ excited state manifold $|e_m\rangle$ $(m = 0, \pm1)$. We treat the problem in the Coulomb gauge and in the dipolar electric approximation [7]. We use in the following the standard decomposition of a field $E(\boldsymbol{r},t)$ in positive/negative frequency components $\boldsymbol{E}^{(\pm)}$, *i.e.* $\boldsymbol{E}(\boldsymbol{r},t) = {\rm e}^{i\omega_{\rm L}t}\boldsymbol{E}^{(-)}(\boldsymbol{r},t) + {\rm e}^{-i\omega_{\rm L}t}\boldsymbol{E}^{(+)}(\boldsymbol{r},t)$, with the same convention for the atomic dipoles in the rotating frame. Note that $\hat{d}_m^{(-)} = d|e_m\rangle\langle g|$ and $\hat{d}_m^{(+)} = \left(\hat{d}_m^{(-)}\right)^\dagger$ are respectively "raising" and "lowering" operators. In the following, all equations will be given for the positive frequency component and we omit the subscript $(+)$ in the averages to alleviate notations.

For a collection of $N$ static dipoles fixed at positions $\{\boldsymbol{r}_i\}_{i=1,\cdots,N}$, the total average electric field $\boldsymbol{E} = \langle\hat{\boldsymbol{E}}^{(+)}\rangle$ can be expressed as [5, 8]

$$\boldsymbol{E}(\boldsymbol{r}) = \boldsymbol{E}_{\rm L}(z) + \frac{1}{\varepsilon_0}\sum_{i=1}^{N}\bar{\bar{G}}(\boldsymbol{r}-\boldsymbol{r}_i)\cdot\boldsymbol{d}_i, \tag{18}$$

with the incident field $\boldsymbol{E}_{\rm L}(z) = E_{\rm L}{\rm e}^{ik_{\rm L}z}\boldsymbol{\varepsilon}_{\rm L}$, the average dipole $\boldsymbol{d}_i = \langle\hat{\boldsymbol{d}}_i^{(+)}\rangle$, and the so-called dyadic Green function

$$G_{m,m'}(\boldsymbol{s}) = \frac{k_{\rm L}^3}{6\pi}\mathcal{G}_{mm'}\left[k_{\rm L}\boldsymbol{s}\right] - \frac{1}{3}\delta_{m,m'}\delta(\boldsymbol{s}), \tag{19}$$

$$\bar{\bar{\mathcal{G}}}\left[\boldsymbol{x}\right] = \frac{3{\rm e}^{{\rm i}x}}{2}\left[\frac{\bar{\bar{\mathcal{D}}}(\underline{\boldsymbol{x}})}{x} + \bar{\bar{\mathcal{Q}}}(\underline{\boldsymbol{x}})\left(\frac{\rm i}{x^2} - \frac{1}{x^3}\right)\right]. \tag{20}$$

We have introduced the dipolar and quadrupolar tensors

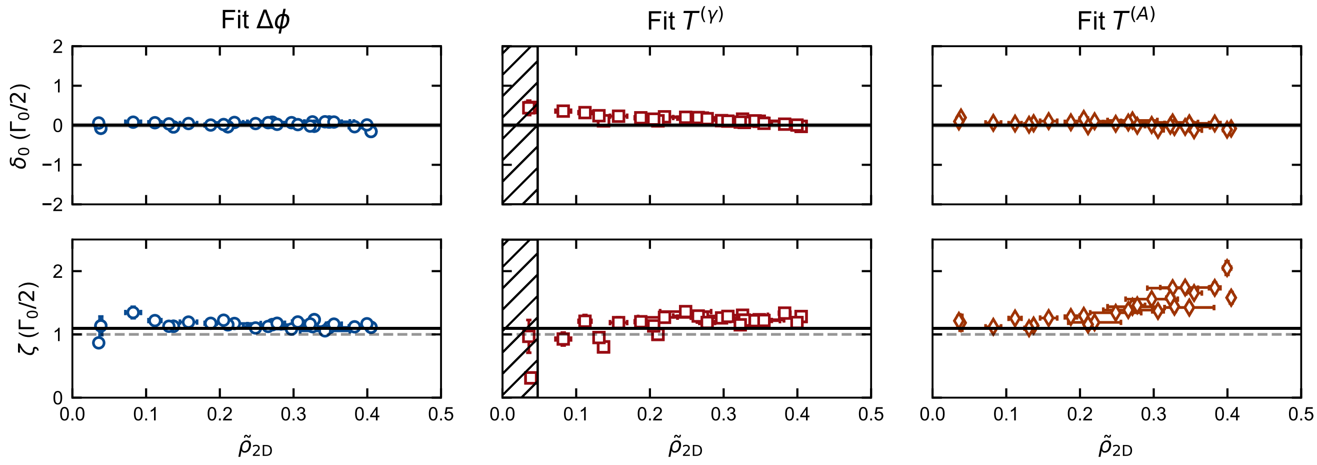


FIG. S2. Result of Lorentzian fits to Eq. (16) and Eq. (17). The reference center frequency $\omega_0$ is calibrated with the mean of the low-density phase-shift data. The shaded regions indicate the uncertainty on the center frequency. The hatched regions indicate the parameter range where the contrast analysis is dominated by imaging noise and not significative.

defined as

$$\mathcal{D}_{mm'}(\underline{\boldsymbol{x}}) = \delta_{mm'} - \frac{x_m x_{m'}}{x^2}, \quad (21)$$

$$\mathcal{Q}_{mm'}(\underline{\boldsymbol{x}}) = \delta_{mm'} - \frac{3x_m x_{m'}}{x^2}, \quad (22)$$

and the notation $\underline{\boldsymbol{x}} = \boldsymbol{x}/x$ for the orientation of the vector $\boldsymbol{x}$.

The steady-state equations of motion for the expected dipoles $\{\boldsymbol{d}_i^{(+)}\}_{i=1,\cdots,N}$ are

$$\boldsymbol{d}_i = \alpha_0(\widetilde{\delta}) \left[ \varepsilon_0 \boldsymbol{E}_{\mathrm{L}}(z_i) + \sum_{j\neq i} \bar{\bar{\mathcal{G}}}(\boldsymbol{r}_{ij}) \cdot \boldsymbol{d}_j \right], \quad (23)$$

with $\boldsymbol{r}_{ij} = \boldsymbol{r}_i - \boldsymbol{r}_j$ and with the single-atom polarizability

$$\alpha_0(\widetilde{\delta}) = -\frac{6\pi}{k_{\mathrm{L}}^3 \left(\widetilde{\delta} + \mathrm{i}\right)}. \quad (24)$$

The set of equations (18,23) is known as the "Fundamental Equations of Multiple Scattering" [9] or sometimes as the Foldy-Lax equations in the litterature [10, 11].

### B. Coupled dipole simulations

To solve numerically the Fundamental Equations of Multiple Scattering Eqs. (18) and (23), we first adopt the dimensionless notations introduced by Chomaz *et al.* [8],

$$X_{i,m} = -\frac{k_{\mathrm{L}}^3}{6\pi\varepsilon_0 E_{\mathrm{L}}} d_{i,m}^{(+)}, \qquad Y_{i,m} = \mathrm{e}^{\mathrm{i}k_{\mathrm{L}} z_i} \varepsilon_{\mathrm{L},m}, \quad (25)$$

with $m = x, y, z$ indexing the components of the mean dipoles. With these notation, we rewrite the Fundamental Equations of Multiple Scattering as a linear system,

$$\boldsymbol{M} \cdot \boldsymbol{X} = \boldsymbol{Y}. \quad (26)$$

Here $M$ is a $3N \times 3N$ matrix with entries

$$M_{i,m;j,m'} = \begin{cases} \delta + \mathrm{i}, & i = j, m = m' \\ \sum_{j\neq i} \mathcal{G}_{mm'}(\boldsymbol{r}_{ij}), & i \neq j \end{cases}. \quad (27)$$

We evaluate $\boldsymbol{M}$ numerically by first drawing the $N$ random positions using rejection sampling and a uniform probability distribution in a disk of radius $R$ chosen to match the desired surface density $\rho_{2\mathrm{D}} = N/(\pi R^2)$. The $z$ coordinates are also drawn randomly but from a Gaussian distribution of root-mean-square width $\Delta z$. In practice, we use $N = 12000$ atoms, which is on the same order of magnitude as the experimental atom numbers (up to $4.5 \times 10^4$). From the inverse matrix $\boldsymbol{M}^{-1}$ calculated numerically, we obtain the complex transmission coefficient [8]

$$t \simeq 1 - \frac{\mathrm{i}k_{\mathrm{L}}\rho_{2\mathrm{D}}}{E_{\mathrm{L}} N} \sum_i \frac{d_{i,\alpha}}{\epsilon_0} \mathrm{e}^{-\mathrm{i}k_{\mathrm{L}} z_i} \quad (28)$$

for this particular realization of the disorder. We then average this result over the disorder by repeating the same procedure typically three times.

## IV. INDEPENDENT SCATTERER MODEL FOR A SLAB GEOMETRY

### A. Propagation equation for the electric field

With the mean particle $\boldsymbol{\rho}(\boldsymbol{r}) = \sum_{i=1}^N \delta(\boldsymbol{r} - \boldsymbol{r}_i)$ and electric polarization $\boldsymbol{P}(\boldsymbol{r}) = \sum_{i=1}^N \delta(\boldsymbol{r} - \boldsymbol{r}_i)\boldsymbol{d}_i$ densities, we rewrite Eq. (18) determining the local electric field as

$$\boldsymbol{E}(\boldsymbol{r}) = \boldsymbol{E}_{\mathrm{L}}(z) + \frac{1}{\varepsilon_0} \int d^3\boldsymbol{r}' \, \bar{\bar{G}}(\boldsymbol{r} - \boldsymbol{r}') \cdot \boldsymbol{P}(\boldsymbol{r}'). \quad (29)$$

Morice *et al.* [5] establish a hierarchy of equations one-body to two-body observables, two-body to three-body observables, etc., which continues until $N-$body observables. Here we truncate the hierarchy to the lowest non trivial order neglecting the mutual influences among different dipoles,

$$\boldsymbol{P}(\boldsymbol{r}) \approx \alpha_0\big(\widetilde{\delta}\big)\rho(\boldsymbol{r})\varepsilon_0\boldsymbol{E}(\boldsymbol{r}). \tag{30}$$

This approximation corresponds to the *independent scatterers approximation* in the language of multiple scattering theory [12]. Each scatterer is visited only once by a given incident photon, but arbitrary numbers of subsequent scattering events by different scatterers are taken into account. Inserting in Eq. (29), we obtain a closed integro-differential equation for the steady electric field in the approximation of independent scatterers,

$$\boldsymbol{E}(\boldsymbol{r}) = \boldsymbol{E}_{\mathrm{L}}(z) + \alpha_0\big(\widetilde{\delta}\big)\int d^3\boldsymbol{r'}\,\bar{\bar{G}}\big(\boldsymbol{r}-\boldsymbol{r'}\big)\cdot\rho(\boldsymbol{r'})\boldsymbol{E}(\boldsymbol{r'}). \tag{31}$$

We consider a slab geometry characterized by the density profile $\rho(z) = \rho_{2\mathrm{D}}f(z)$, uniform along the $x-y$ directions and varying according to a given profile $f(z)$ in the $z$ direction. The mean electric polarization and electric field depend only on the $z$ coordinate by translational invariance. The integration over the transverse $x, y$ coordinates in Eq. (31) can be performed analytically using the formula

$$\int d^3\boldsymbol{r'}\,\overline{\overline{G}}\left[k_{\mathrm{L}}(\boldsymbol{r}-\boldsymbol{r'})\right]\cdot\boldsymbol{V}(z') = \frac{\mathrm{i}k_{\mathrm{L}}}{2}\int dz'\mathrm{e}^{\mathrm{i}k_{\mathrm{L}}(|z-z'|-z+z')}\boldsymbol{V}_{\perp}(z') - V_z(0)\,\boldsymbol{e}_z \tag{32}$$

valid for a vector field $\boldsymbol{V}(z)$ that depends only on $z$, with $\boldsymbol{V}_{\perp} = V_x\boldsymbol{e}_x + V_y\boldsymbol{e}_y$. Applying Eq. (32) to the average electric field in Eq. (31) and using $k_{\mathrm{L}}\alpha_0\big(\widetilde{\delta}\big)\rho_{2\mathrm{D}} = -6\pi\widetilde{\rho}_{2\mathrm{D}}/(\widetilde{\delta}+\mathrm{i})$, we obtain Eq. (3) in the main text.

Eq. (32) can be established by a direct calculation, or from a more physical argument. The propagation of the electric field $\boldsymbol{E}$ is governed by the Helmholtz equation (here, in the Coulomb gauge),

$$-\big(k_{\mathrm{L}}^2+\Delta\big)E_i + \partial_i\Big(\sum_j\partial_jE_j\Big) = \frac{k_{\mathrm{L}}^2}{\varepsilon_0}P_i, \tag{33}$$

with a general solution $E_i(\boldsymbol{r}) = \int d^3\boldsymbol{r'}G_{ij}(\boldsymbol{r}-\boldsymbol{r'})P_j(\boldsymbol{r'})$. and with $\bar{\bar{G}}$ the dyadic Green function. When the transverse components $E_+\mathrm{e}^{\mathrm{i}k_{\mathrm{L}}z}, P_+\mathrm{e}^{\mathrm{i}k_{\mathrm{L}}z}$ depend only on $z$, the propagation equation reduces to the one-dimensional Helmholtz equation, with general solution $E_+(z) = \int dz'g_{1\mathrm{D}}(z-z')P_+(z')\mathrm{e}^{-\mathrm{i}k_{\mathrm{L}}(z-z')}$ and Green function $g_{1\mathrm{D}}(x) = \mathrm{i}/(2k_{\mathrm{L}})\mathrm{e}^{\mathrm{i}k_{\mathrm{L}}|x|}$. The 3D and 1D solutions are compatible with each other if and only if

$$\int dx'dy'\,G_{++}(\boldsymbol{r}-\boldsymbol{r'}) = g_{1\mathrm{D}}(z-z'). \tag{34}$$

This formula reproduces Eq. (32) in the special case $\boldsymbol{V} = V_+(z)\boldsymbol{e}_+$.

### B. Thick samples

For thick samples with $k_{\mathrm{L}}\Delta z \gg 1$, the reflected component is negligible and the propagation equation reduces to

$$E_+(z) \approx E_{\mathrm{L}} - \frac{\mathrm{i}3\pi\widetilde{\rho}_{2\mathrm{D}}}{\widetilde{\delta}+\mathrm{i}}\int_{-\infty}^{z}dz'\,f(z')E_+(z') \tag{35}$$

with $\boldsymbol{E} = E_+\boldsymbol{\varepsilon}_{\mathrm{L}}$ and $6\pi\widetilde{\rho}_{2\mathrm{D}}$ corresponds to the usual resonant optical depth. Differentiating with respect to $z$, one gets the differential equation

$$\frac{1}{E_+}\frac{dE_+}{dz} \approx -\frac{\mathrm{i}3\pi\widetilde{\rho}_{2\mathrm{D}}}{\widetilde{\delta}+\mathrm{i}}f(z), \tag{36}$$

whose solution is a "generalized" Beer-Lambert formula,

$$\frac{E_+(z)}{E_{\mathrm{L}}} \approx \exp\left[-\frac{\mathrm{i}3\pi\widetilde{\rho}_{2\mathrm{D}}}{\widetilde{\delta}+\mathrm{i}}\int_{-\infty}^{z}dz'\,f(z')\right]. \tag{37}$$

Taking a Gaussian $f(z)$ (see main article), we find a complex transmission

$$t_{\mathrm{BL}} = \frac{E_+(z\to+\infty)}{E_{\mathrm{L}}} \approx \exp\left(-3\pi\widetilde{\rho}_{2\mathrm{D}}\frac{\mathrm{i}\widetilde{\delta}+1}{\widetilde{\delta}^2+1}\right). \tag{38}$$

### C. Thin samples

In the opposite case of a thin membrane with $k_{\mathrm{L}}\Delta z \to 0$, $f(z)$ can be treated as a Dirac delta function. From Eq. (3) in the main text and requiring the continuity of $E_+$ across the medium at $z=0$, we obtain complex transmission and reflection coefficients

$$t_{2\mathrm{D}} = \frac{\widetilde{\delta}+\mathrm{i}}{\widetilde{\delta}+\mathrm{i}\,(1+3\pi\widetilde{\rho}_{2\mathrm{D}})}, \tag{39}$$

$$r_{2\mathrm{D}} = -\frac{3\pi\widetilde{\rho}_{2\mathrm{D}}}{\widetilde{\delta}+\mathrm{i}\,(1+3\pi\widetilde{\rho}_{2\mathrm{D}})}. \tag{40}$$

### D. Lineshape for arbitrary thickness

Outside of the limiting cases studied above, we solve the propagation Eq. (31) numerically. Figure S3 shows the evolution of the lineshape for $\widetilde{\rho}_{2\mathrm{D}} = 0.5$. Although the lineshape is symmetric in the limiting cases $k_{\mathrm{L}}\Delta z \to 0$ or $+\infty$, it is asymmetric in general with a maximal "distortion" around $k_{\mathrm{L}}\Delta z \sim 1$. As emphasized in the main text, this asymmetry stems from an etalon effect where the reflected and transmitted waves interfere with each other inside the medium. The interference disappears in the limits $\Delta z \to 0, +\infty$ for different reasons. When $\Delta z \to 0$, the etalon has zero thickness and when $\Delta z \to +\infty$, the reflected component vanishes.

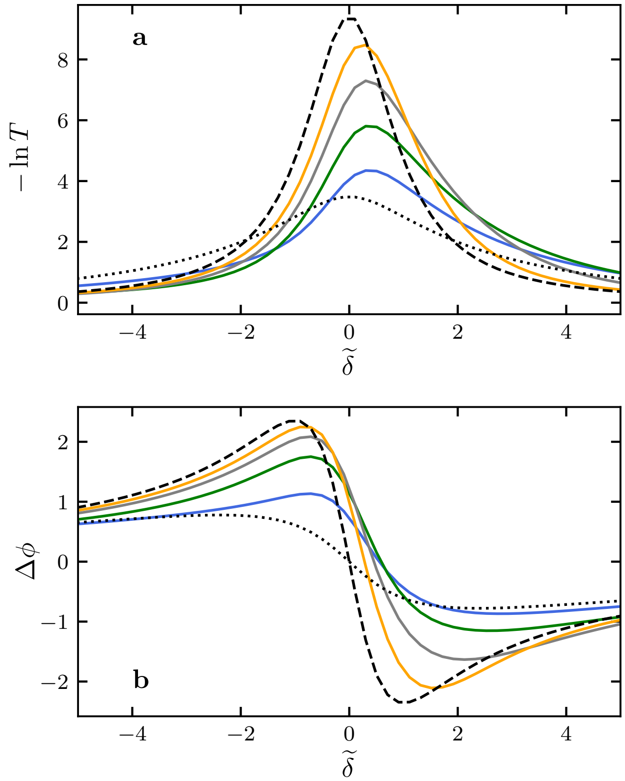


FIG. S3. Optical depth $-\ln T$ (**a**) and phase shift $\Delta\phi$ (**b**) for the independent scatterer model and the Gaussian slab geometry. The solid lines correspond to the numerical calculation for $k_{\mathrm{L}}\Delta z = 0.25, 0.5, 1, 2$ from bottom to top. The dotted and dashed lines show the limiting 2D ($k_{\mathrm{L}}\Delta z \to 0$) and 3D cases 2D ($k_{\mathrm{L}}\Delta z \to +\infty$). For all plots, the surface density is $\widetilde{\rho}_{2\mathrm{D}} = 0.5$.

## V. PARASITIC EFFECTS IN INTENSITY TRANSMISSION MEASUREMENTS

### A. Off-axis scattering

Any imaging system has a finite numerical aperture, which means that it collects the electric field at locations (slightly) away from the propagation axis. Here we attempt to evaluate the difference between the imaging signal and the "true" intensity transmission coefficient defined as the ratio of the intensity of the forward scattered wave to the intensity of the incident wave,

$$T = \frac{\left|E_+(z \to +\infty)\right|^2}{\left|E_{\mathrm{L}}\right|^2}. \tag{41}$$

As before, we assume that the polarisability of the medium is along the incident polarization and only depends on $z$, $\boldsymbol{P}(z) = P(z)\boldsymbol{\varepsilon}_{\mathrm{L}}$, and neglect edge effects due to the finite transverse extent of the medium.

We consider observation distances large compared to any dimension of the medium and restrict ourselves to a narrow cone around the $z$ axis. Using cylindrical coordinates with $\boldsymbol{r} - \boldsymbol{r'} = \boldsymbol{\rho} + (z - z')\boldsymbol{e}_z$, the dyadic Green function in Eq. (20) can be approximated as

$$\bar{\bar{\mathcal{G}}} \approx \frac{3\mathrm{e}^{\mathrm{i}k_{\mathrm{L}}\left[|z| - \mathrm{sign}(z)z'\right] + \mathrm{i}\frac{k_{\mathrm{L}}\rho^2}{2|z|}}}{2|z|}(1 - \underline{\boldsymbol{r}} \otimes \underline{\boldsymbol{r}}), \tag{42}$$

with $\underline{\boldsymbol{r}} = \boldsymbol{r}/r$. Inserting this expression in Eq. (29), we obtain the expression of the scattered electric field far from the atomic medium,

$$\boldsymbol{\mathcal{E}}(\boldsymbol{r})\mathrm{e}^{-\mathrm{i}k_{\mathrm{L}}z} = E(z)\boldsymbol{\varepsilon}_{\mathrm{L}} + (\boldsymbol{\varepsilon}_{\mathrm{L}} \cdot \underline{\boldsymbol{r}})\left[E_{\mathrm{L}} - E(z)\right]\underline{\boldsymbol{r}} \tag{43}$$

with the forward scattered field $E(z)$ obeying Eq. (3) in the main article. The optical intensity is proportional to $|\boldsymbol{\mathcal{E}}(\boldsymbol{r})|^2 = \left|E(z)\right|^2 + \left|\boldsymbol{\varepsilon}_{\mathrm{L}} \cdot \underline{\boldsymbol{r}}\right|^2 \left\{\left|E_{\mathrm{L}}\right|^2 - \left|E(z)\right|^2\right\}$, which can be rewritten as

$$\frac{|\boldsymbol{\mathcal{E}}(\boldsymbol{r})|^2}{|E_{\mathrm{L}}|^2} = T + \left|\boldsymbol{\varepsilon}_{\mathrm{L}} \cdot \underline{\boldsymbol{r}}\right|^2 \Big(1 - T\Big). \tag{44}$$

We now consider the total flux of photons $\Phi$ collected by the imaging system, modeled as an ideal front lens $\mathcal{L}$ of radius $R$ and focal distance $f$ located at $z = f$. We find that

$$\Phi = \frac{1}{\hbar\omega_{\mathrm{L}}} \int_{\mathcal{L}} d^2\boldsymbol{\rho}\, \varepsilon_0 c \left|\boldsymbol{\mathcal{E}}(\boldsymbol{r})\right|^2, \tag{45}$$

$$= \Phi_{\mathrm{L}} \left[T + (1 - T)\, \frac{1}{\pi R^2} \int_{\mathcal{L}} d^2\boldsymbol{\rho} \left|\boldsymbol{\varepsilon}_{\mathrm{L}} \cdot \underline{\boldsymbol{r}}\right|^2\right]. \tag{46}$$

The quantity $\Phi_{\mathrm{L}} = \varepsilon_0 c \left|E_{\mathrm{L}}\right|^2 \pi R^2/(\hbar\omega_{\mathrm{L}})$ is the amount of energy in the incident plane wave collected by the imaging system divided by the energy of a single photon. The quantity $T\Phi_{\mathrm{L}}$ is the amount collected from the transmitted wave. Flux conservation (or the optical theorem

in the language of scattering theory) tells us that the total flux from the scattered component (excluding the forward direction) must sum up to $\Phi_L(1-T)$. The remaining term in Eq. (46) corresponds to the fraction $F$ of the scattered flux collected by the imaging system,

$$F(\Theta) = \frac{1}{\pi R^2}\int_{\mathcal{L}} d^2\boldsymbol{\rho} \left|\boldsymbol{\varepsilon}_L \cdot \underline{\boldsymbol{r}}\right|^2 = \frac{1}{2}\left[1 - \frac{\ln(1+\Theta^2)}{\Theta^2}\right], \tag{47}$$

with $\tan\Theta = R/f$. The limit $R \to +\infty$ ($\Theta \to \infty$) corresponds to a front lens much larger than the distance to the sample. In that situation, almost all the light emitted in the $z > 0$ half space is collected, and $F \to 1/2$ as can be expected. The opposite limit $R \to 0$ corresponds to an actual imaging system. This leads to $F \approx \Theta^2/4$ and to an apparent transmission as recorded by the imaging system,

$$T_{\rm app} = \frac{\Phi}{\Phi_L} \simeq T + \frac{\Theta^2}{4}(1-T). \tag{48}$$

### B. Imaging noise

Photons collected by the camera are converted to digital counts. The optical intensity-counts conversion coefficient is given by

$$\kappa = \frac{\eta_{\rm cam.} \cdot (A/M^2) \cdot t_p}{\hbar\omega_0} \tag{49}$$

where $\eta_{\rm cam.}$ is the quantum efficiency of the camera at the imaging wavelength $\lambda_0$, $A$ is the pixel area, $M$ is the magnification of the imaging system, $t_p$ is the illumination time. The maximum number of counts in a reference region away from the atomic cloud is large, $C^{\max} = \kappa I_L \gg 1$, while the number of counts in a region inside the atomic medium $C^{\min} \simeq C^{\max} e^{-D_0} \ll 1$ is typically very low. As a result, we have to worry about camera noise in the atom region.

For a given image, the digital signal per pixel in the ROI containing the atoms can be expressed as

$$C^{(\rm at)} \approx \delta C^{(\rm at)} + \kappa I_t, \tag{50}$$

with $\delta C^{(\rm at)}$ the camera read-out noise. Commonly, the digital signal is in fact given by $C_0 + C^{(\rm at)}$, where $C_0$ is a constant and almost uniform offset (usually added at the level of the output register of the camera). We assume that the offset $C_0$ is removed through signal processing, also a common procedure. The approximate symbol in Eq. (50) means that we neglect the intensity variations across each pixel to simplify the discussion. Because the counts can only be positive, the stochastic variable $\delta C^{(\rm at)}$ has a non-zero expectation value over many realizations. We assume here that it follows Poisson statistics, so that $\overline{\delta C^{(\rm at)}} = \sigma/\eta$ with $\sigma$ the noise standard deviation specified by the camera manufacturer. Similarly, the signal from the reference region can be written

$$C^{(\rm ref)} \approx \delta C^{(\rm ref)} + \kappa I_L. \tag{51}$$

The "experimental transmission" is then defined as

$$T_{\rm exp,1\,real.} = \frac{\widetilde{C}^{(\rm at)}}{\widetilde{C}^{(\rm ref)}} \approx \frac{I_t}{I_L} + \frac{\delta C^{(\rm at)}}{\kappa I_L} - \frac{I_t}{I_L}\frac{\delta C^{(\rm ref)}}{\kappa I_L}, \tag{52}$$

where we use $\kappa I_L \gg \delta C^{(\rm ref)}$ to perform a Taylor expansion with $\delta C^{(\rm at/ref)}$ as small parameters. Averaging over several realizations of the noise and assuming that $\overline{\delta C^{(\rm ref)}} = \overline{\delta C^{(\rm at)}} \equiv \overline{\delta C}$, we find another correction to the experimental "transmission",

$$T_{\rm exp} \approx T + \left(T_{\rm noise} + \frac{\Theta^2}{4}\right)(1-T), \tag{53}$$

with a noise factor

$$T_{\rm noise} = \frac{\overline{\delta C}}{\kappa I_L}. \tag{54}$$

This model is compared to our experimental data in the main article and in Fig. S4a. As a complement, we compare the model in Fig. S4b to another set of experiments with $^{87}$Rb atoms reported in [13]. The model parameters are taken from Table I –listing experimental values and manufacturer specifications– *without any free parameter*. For both comparisons, we use the resonant Beer-Lambert law $T = e^{-6\pi\widetilde{\rho}_{2D}}$ for simplicity. The model reproduces the observed plateau which is mostly due to camera noise, with off-axis scattering giving a smaller but not completely negligible contribution. The model also apparently overestimates the initial slope before reaching the plateau. We believe that this effect comes from using the Beer-Lambert law for $T$, and could be improved by upgrading to a better model or using the transmission measured in interference experiments, uncontaminated by noise or by off-axis scattering. Unfortunately, the latter are not available for the experiments of [13] and we are not able to perform coupled dipole simulations free of finite size effects at the densities reached in this experiment (significantly higher than in our work).


[1] C.-L. Hung, X. Zhang, N. Gemelke, and C. Chin, Nature **470**, 236 (2011).

[2] T. Yefsah, R. Desbuquois, L. Chomaz, K. J. Günter, and J. Dalibard, Phys. Rev. Lett. **107**, 130401 (2011).

[3] N. Prokof'ev and B. Svistunov, Phys. Rev. A **66**, 043608 (2002).

| Ref. | Atom | $\lambda_0$ | $I_L$ | $t_{pulse}$ | $\kappa$ | $N^{max}_{ph-\bar{e}}$ | $T_{noise}$ |
|---|---|---|---|---|---|---|---|
| this work | $^{174}$Yb | 398.9 nm | 12.6 mW/cm$^2$ | 5 $\mu$s | 0.87 | 273 | 0.073 |
| [13] | $^{87}$Rb | 780 nm | 0.32 mW/cm$^2$ | 10 $\mu$s | 47 | 167 | 0.020 |

| Ref. | Camera | quantum eff. $\eta_{cam.}$ ($\bar{e}$/ph.) | pixel size $p$ | noise $\sigma$ [$\bar{e}$/px] | magnification $M$ |
|---|---|---|---|---|---|
| this work | PCO PixelFly USB | $\approx 0.4$ | 6.5 $\mu$m | $\approx 8$ | 14 |
| [13] | Roper Scientific PIXIS 1024 BR | $\approx 0.9$ | 13 $\mu$m | $\approx 3$ | 11 |

TABLE I. Relevant experimentat figures for the experiments reported in this work and in [13].

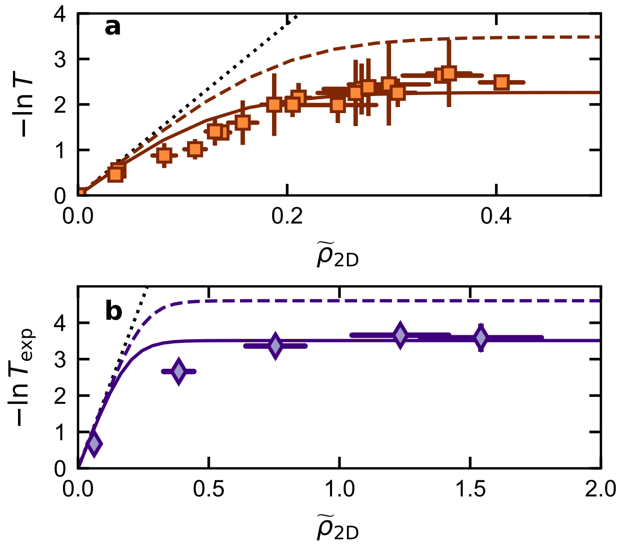


FIG. S4. Comparison between the model including off-axis scattering and camera noise for our experiments with $^{174}$Yb atoms (**a**) and for the experiments with $^{87}$Rb atoms reported in [13] (**b**). The dotted line is the Beer-Lambert law on resonance, $e^{-6\pi\widetilde{\rho}_{2D}}$. The solid line improves on the Beer-Lambert model by including off-axis scattering and camera noise [Eq. (53)]. For comparison, the dashed line show the same model but including only off-axis scattering (*i.e.* setting $T_{noise} = 0$) in Eq. (53).


[4] I. Bloch, J. Dalibard, and W. Zwerger, Rev. Mod. Phys. **80**, 885 (2008).

[5] O. Morice, Y. Castin, and J. Dalibard, Phys. Rev. A **51**, 3896 (1995).

[6] P. C. Bons, R. de Haas, D. de Jong, A. Groot, and P. van der Straten, Phys. Rev. Lett. **116**, 173602 (2016).

[7] C. Cohen-Tannoudji, G. Grynberg, and J. Dupont-Roc, *Atom Photon Interactions*, Atomic and Molecular Physics (John Wiley & Sons, 1992).

[8] L. Chomaz, L. Corman, T. Yefsah, R. Desbuquois, and J. Dalibard, New J. Phys. **14**, 055001 (2012).

[9] L. L. Foldy, Phys. Rev. **67**, 107 (1945).

[10] M. Lax, Rev. Mod. Phys. **23**, 287 (1951).

[11] M. Lax, Phys. Rev. **85**, 621 (1952).

[12] W. Guerin, M. T. Rouabah, and R. Kaiser, J. Mod. Opt. **64**, 895 (2017).

[13] L. Corman, J. L. Ville, R. Saint-Jalm, M. Aidelsburger, T. Bienaimé, S. Nascimbène, J. Dalibard, and J. Beugnon, Phys. Rev. A **96**, 053629 (2017).
